# Supplementary material for: PolarRec: Radio Interferometric Data Reconstruction with Polar Coordinate Representation
Source: arXiv:2308.14610 source file (2023-11-27)
Supplement: Supplementary file 1 [file X_suppl.tex]

\clearpage
\setcounter{page}{1}
\maketitlesupplementary

This document provides supplementary information that
is not included in our main paper due to space limitation: Section A further explains the visibility distance in our method. Section B describes the details of our experiments.

\setcounter{section}{0}

\section{Additional Explanation of Visibility Distance}
The visibility distance is between real and predicted visibility in complex values, reflecting the amplitude and phase information of visibility data.

In radio interferometry imaging process, amplitude represents the intensity or energy of a signal, and corresponds to the strength with which an image responds to the 2D sinusoidal wave at a specific frequency \cite{jiang2021focal}. Phase encodes the positional information of signal components \cite{oppenheim1981importance}, helping reconstruct the spatial relationships and structures within the image data.

The magnitude of a vector in a 2D plane, given by \( \sqrt{A^2 + B^2} \), corresponds to the absolute value of the complex number.
The magnitude of \( \vec{p_r} \) is \( |\vec{p_r}| = \sqrt{A_r^2 + B_r^2} \), which is the same as the amplitude of \( V_r(u, v) \).
Similarly, The magnitude of \( \vec{p_p} \), \( |\vec{p_p}| = \sqrt{A_p^2 + B_p^2} \) represents the amplitude of \( V_p(u, v) \). The phase of a complex number \( A + iB \) is the angle between the vector and the real axis in the complex plane, typically measured in radians or degrees.
This angle can be calculated using the arctangent function: \( \theta = \arctan\left(\frac{B}{A}\right) \).  For \( \vec{p_r} \), the angle \( \theta_r = \arctan\left(\frac{B_r}{A_r}\right) \) represents the phase of \( V_r(u, v) \).
For \( \vec{p_p} \), \( \theta_p = \arctan\left(\frac{B_p}{A_p}\right) \) corresponds to the phase of \( V_p(u, v) \).

The magnitude of the vectors \( |\vec{p_r}| \) and \( |\vec{p_p}| \) represent the amplitudes of the complex visibility values, reflecting the strength or intensity of the signal components in the spatial frequency domain.
The angles \( \theta_r \) and \( \theta_p \) of the vectors correspond to the phases of the complex visibility values, indicating the positional information and structural arrangement of the image components. As a result, the single point visibility distance defined by $d(\vec{p_r}, \vec{p_p})$ covers information from both amplitude and phase.

\section{Additional Experiment Details}
\subsection{Implementation Details of PolarRec}
We provide our demo code in the supplementary material. All the code we used for the experiments will be public if the paper is published. In our implementation of PolarRec, we use a 2-layer MLP with a Leaky ReLU activation in the intra-group encoder, followed by an adaptive average pooling layer. The inter-group encoding is done by a Transformer encoder. We then use an 8-layer MLP in the conditioned neural field, and only the first 8 output tokens with the dimension of 1024 from the Transformer encoder are used to condition this 8-layer MLP. We show the details of the FiLM conditioning network and PorlarRec encoder in our model in table \ref{FiLMConditioning} and table \ref{PolarRecEncoder}. 

Our model is trained with Adam with $lr = 0.0001, \beta_1 = 0.9, \beta_2 = -0.999, \text{eps} = 1 \times 10^{-8}, \text{weight decay} = 0$. The two scaling factors $\alpha$ and $\beta$ in the Radial Visibility Loss are both set to 1. The model for overall comparison is trained with batch\_size = 32 and group\_size = 32.

\begin{table*}[h]
\centering
\begin{tabular}{|l|l|}
\hline
\textbf{Component}               & \textbf{Details}                                      \\ \hline
Positional Embedding                       & PE\_Module: Fourier Encoding                                            \\ \hline
\multirow{4}{*}{Layers (FiLMLinear x7)} & Linear: in\_features=258 (for the first layer), 256 (for subsequent layers), \\ & out\_features=256, bias=True (first layer only) \\
                                        & Activation1: LeakyReLU (negative\_slope=0.01)       \\
                                        & Activation2: LeakyReLU (negative\_slope=0.01)       \\
                                        & Film1: Linear, in\_features=1024, out\_features=256, bias=True \\
                                        & Film2: Linear, in\_features=1024, out\_features=256, bias=True \\ \hline
Activations                      & ModuleList containing 7 ReLU activations             \\ \hline
Final Layer (FiLMLinear)        & \begin{tabular}[c]{@{}l@{}}Linear: in\_features=256, out\_features=2, bias=True\\ Activation1: LeakyReLU (negative\_slope=0.01)\\ Activation2: LeakyReLU (negative\_slope=0.01)\\ Film1: Linear, in\_features=1024, out\_features=2, bias=True\\ Film2: Linear, in\_features=1024, out\_features=2, bias=True\end{tabular} \\ \hline
\end{tabular}
\caption{FiLM Conditioning Component Structure}
\label{FiLMConditioning}
\end{table*}

\begin{table*}[h]
\centering
\begin{tabular}{|l|l|}
\hline
\textbf{Component} & \textbf{Details} \\ \hline
Linear Embedding for Visibility Values & Sequential (Linear: in\_features=2, out\_features=254, bias=True) \\ \hline
\begin{tabular}[c]{@{}l@{}}
Intra-group Encoding
\end{tabular} & 
\begin{tabular}[c]{@{}l@{}}
Sequential (Linear: in\_features=512, out\_features=256, bias=True, \\LeakyReLU: negative\_slope=0.01,\\ Linear: in\_features=256, out\_features=512, bias=True) \\
AdaptiveAvgPool2d, output\_size=(1660 // group\_size, 512) \\
Dropout, p=0.0
\end{tabular} \\ \hline
Inter-group Encoding & \begin{tabular}[c]{@{}l@{}}Transformer with 4 sets of module lists, each containing:\\ - Residual with PreNorm and Attention (to\_qkv Linear: in\_features=512, \\ out\_features=1536, bias=False, to\_out Sequential: Linear in\_features=512, \\ out\_features=512, bias=True)\\ - Residual with PreNorm and FeedForward (Sequential: Linear in\_features=512, \\ out\_features=512, bias=True)\end{tabular} \\ \hline
Output Token Heads & \begin{tabular}[c]{@{}l@{}}Module list containing 8 Sequential modules, each with:\\ - LayerNorm: (512,), eps=1e-05, elementwise\_affine=True\\ - Linear: in\_features=512, out\_features=1024, bias=True\end{tabular} \\ \hline
\end{tabular}
\caption{PolarRec Encoder Component Structure}
\label{PolarRecEncoder}
\end{table*}

\begin{table*}[h]
\centering
\caption{Dataset Information.}
\begin{tabular}{|l|c|c|c|}
\hline
\textbf{Dataset} & \textbf{Total Size} & \textbf{Test Set Size} \\ \hline
Merging Galaxies (MG) & 1853 & 370 \\ \hline
In-between Round Smooth Galaxies (IRSG) & 2027 & 405 \\ \hline
Unbarred Tight Spiral Galaxies (UTSG) & 1829  & 365 \\ \hline
Edge-on Galaxies with Bulge (EGB) & 1873 & 374 \\ \hline
\end{tabular}
\label{datasets}
\end{table*}

\subsection{Baseline Details}
\subsubsection{CLEAN}
\textsc{CLEAN} \cite{hogbom1974aperture} facilitates the extraction of the original image, denoted as \( I(l, m) \), from the observed visibilities \( V(u, v) \) and the telescope array configuration \( W(u, v) \). This process can be mathematically expressed as a Fourier inversion of the product of \( V(u, v) \) and \( W(u, v) \), leading to the equation \( F^{-1}[V(u, v)W(u, v)] = I(l, m) \ast F^{-1}[W(u, v)] \). The specific arrangement of the telescope array, \( W(u, v) \), yields a point-spread function (PSF) in the image plane, known as the \textit{dirty beam}, represented by \( F^{-1}[W(u, v)] \). The initial image created directly from the complex visibilities, often referred to as the \textit{dirty image}, is the convolution of the dirty beam with the true celestial image \( I(l, m) \) \cite{wu2022neural}. The process of deconvolution in the \textsc{CLEAN} algorithm involves an iterative technique where the peak emission in the dirty image, once convolved with the dirty beam, is systematically subtracted. Throughout this iterative process, a model of the \textit{clean} emission is progressively constructed. In the implementation, we set the threshold to stop iteration to $1 \times 10^{-11}$, $\text{gain}=0.1$, $\text{beam\_size}=4$, $\text{maxIteration}=1 \times 10^5$ for the best performance.

\subsubsection{U-Net}
In the implementation of U-Net, we follow the source code of U-Net with attention and residual blocks for MRI reconstruction \cite{xie2022measurement}. The image size is set to 256 and the number of residual blocks is 2. The attention resolution is set to 20 and the number of heads is set as 4 for the best performance.

\subsubsection{Radionets}
We follow the original source code for Radionets \cite{schmidt2022deep} implementation. We choose $\text{arch\_name = 'SRResNet'}$ as the backbone network for the best performance and set $\text{amp\_phase} = false$ to output the real and imaginary value of visibility data for comparison. 

\subsubsection{Neural Interferometry}
We use the original code of Neural Interferometry \cite{wu2022neural}. The batch size is set to 4 due to the GPU memory capacity limit and the loss type is set as 'spectral' for the best performance. All other settings are the same as the default values in the original code.

\subsection{Dataset Details}
We evaluated the methods on 4 datasets, Merging Galaxies (MG), In-between Round Smooth Galaxies (IRSG), Unbarred Tight Spiral Galaxies (UTSG), and Edge-on Galaxies with Bulge (EGB). For each dataset, we randomly split 20\% of all images for testing, with the remainder being used for training. The details of the datasets are shown in Table \ref{datasets}. Each observation of an image has 1660 sampled visibility points and all the images in our experiments are converted to grayscales for sky intensity information and then scaled to a size of 256 $\times$ 256. Following the methods of Wu et al. \cite{wu2022neural}, we apply the inversed discrete Fourier transform (IDFT) technique to create dirty images out of the visibility data.

% The datasets we used are derived from sources under the DESI Legacy Imaging Surveys \cite{dey2019overview}, integrating contributions from the Beijing-Arizona Sky Survey (BASS) \cite{zou2017project}, the DECam Legacy Survey (DECaLS) \cite{blum2016decam}, and the Mayall z-band Legacy Survey \cite{silva2016mayall}. Specifically, the DECaLS project uses the Dark Energy Camera \cite{flaugher2015dark} on the Blanco 4m telescope, covering both the North Galactic Cap region at $Dec \leq 32^{\circ}$ and the South Galactic Cap region at $Dec \leq 34^{\circ}$ \cite{blum2016decam,dagli2023astroformer}. The DECaLS survey utilizes a method of tiling the sky with 3 separate passes which are slightly shifted in relation to one another, with an approximate offset range of $0.1^{\circ} - 0.6^{\circ}$ \cite{blum2016decam,dagli2023astroformer}. The Beijing-Arizona Sky Survey, utilizing the Steward Observatory’s 2.3m Bok Telescope, mapping a 5000 square degree area of the Northern Galactic Cap \cite{zou2017project, dagli2023astroformer}. The Mayall z-band Legacy Survey focuses on the $Dec \geq 32^{\circ}$ region using the 4-m Mayall telescope \cite{silva2016mayall,dagli2023astroformer}.
